# Supplementary material for: Clustering and spatial distribution of mitochondria in dendritic trees
Source: arXiv:2405.04684 source file (2024-05-07)
Supplement: Supplementary file 1 [file SM.pdf]

# Supplementary Material for: Clustering and spatial distribution of mitochondria in dendritic trees

M. Hidalgo-Soria[1] and E. F. Koslover[1]

[1]*Department of Physics, University of California, San Diego, La Jolla, CA 92093, USA*

## STEADY STATE SOLUTION

Here, we solve Eq. (1) in the main text via recursive methods. Reflection of motile units at terminal tips implies that $\rho^+_{1,j} = \rho^-_{1,j}$ in the distal branches, and this equality propagates through boundary conditions at all junctions. Therefore, we can write the total linear density of motile monomers as $\rho^m_{1,j} = \rho^+_{1,j} + \rho^-_{1,j} = 2\rho^+_{1,j}$. The steady-state equations can then be re-expressed as:

$$\frac{\partial \rho^s_{1,j}}{\partial t} = -2k_b\rho^s_{1,j} + 2k_b\rho^s_{2,j} - vP_{u,j}\rho^m_{1,j}\rho^s_{1,j} = 0, \tag{S.1a}$$

$$\frac{\partial \rho^m_{1,j}}{\partial t} = -vP_{u,j}\rho^m_{1,j}\sum_{i=1}^{\infty}\rho^s_{i,j} - vP_{u,j}(\rho^m_{1,j})^2 + 2k_b\rho^s_{2,j} + 2k_b\rho^s_{1,j} + 2k_b\sum_{i=3}^{\infty}\rho^s_{i,j} = 0, \tag{S.1b}$$

$$\frac{\partial \rho^s_{2,j}}{\partial t} = -vP_{u,j}\rho^m_{1,j}\rho^s_{2,j} + vP_{u,j}\frac{(\rho^m_{1,j})^2}{2} + 2k_b\rho^s_{3,j} - 2k_b\rho^s_{2,j} + vP_{u,j}\rho^m_{1,j}\rho^s_{1,j} = 0, \tag{S.1c}$$

$$\frac{\partial \rho^s_{i,j}}{\partial t} = vP_{u,j}\rho^m_{1,j}(\rho^s_{i-1,j} - \rho^s_{i,j}) + 2k_b\rho^s_{i+1,j} - 2k_b\rho^s_{i,j} = 0. \tag{S.1d}$$

Solving Eq. S.1c gives an expression for $\rho^s_{3,j}$ as:

$$\rho^s_{3,j} = \rho^s_{2,j} + \Big(\rho^s_{2,j} - \rho^s_{1,j} - \frac{\rho^m_{1,j}}{2}\Big)\alpha_j\rho^m_{1,j}, \tag{S.2}$$

where we define $\alpha_j = vP_{u,j}/(2k_b) = vA_u/(2k_b r_j^\gamma)$. Solving Eq. S.1d for $\rho^s_{i+1,j}$ and propagating downward recursively gives a general expression for the linear density of all clusters of size $i > 2$:

$$\rho^s_{i,j} = \rho^s_{2,j} + \Big(\rho^s_{2,j} - \rho^s_{1,j} - \frac{\rho^m_{1,j}}{2}\Big)\sum_{k=1}^{i-2}(\alpha_j\rho^m_{1,j})^k. \tag{S.3}$$

Assuming $|\alpha_j\rho^m_{i,j}| < 1$, we can explicitly sum the partial geometric series to get:

$$\rho^s_{i,j} = \frac{\rho^s_{2,j} - \alpha_j\rho^m_{1,j}\big(\rho^s_{1,j} + \frac{\rho^m_{1,j}}{2}\big) - (\alpha_j\rho^m_{1,j})^{i-1}\big(\rho^s_{2,j} - \rho^s_{1,j} - \frac{\rho^m_{1,j}}{2}\big)}{1 - \alpha_j\rho^m_{i,j}}. \tag{S.4}$$

For a finite total mitochondrial load, the density must vanish at large cluster sizes: $\lim_{i\to\infty}\rho^s_{i,j} = 0$. This implies that the intercept in Eq. (S.4) must be zero:

$$\rho^s_{2,j} = \alpha_j\rho^m_{1,j}\Big(\rho^s_{1,j} + \frac{\rho^m_{1,j}}{2}\Big). \tag{S.5}$$

Solving Eq. (S.1a) then gives:

$$\rho^s_{2,j} = \rho^s_{1,j} + \alpha_j\rho^m_{1,j}\rho^s_{1,j}. \tag{S.6}$$

Together, Eqs. S.4, S.5, S.6 give the full solution for the steady-state density of stationary clusters as a function of the motile density:

$$\rho^s_{1,j} = \frac{\alpha_j(\rho^m_{1,j})^2}{2}, \tag{S.7a}$$

$$\rho^s_{i,j} = \frac{\rho^m_{1,j}}{2}(1 + \alpha_j\rho^m_{1,j})\Big(\alpha_j\rho^m_{1,j}\Big)^{i-1}; \quad i > 1. \tag{S.7b}$$

The motile density $\rho^m_{1,j}$ is obtained by applying the boundary conditions at the root and junctions of the tree. At the root node, we have the boundary condition $\rho^m_{1,0} = 2k_p/v$. For parent $j$ and daughter branches $k, l$, the flux of

motile mitochondria is preserved, *i.e.* $\rho^m_{1,j} = \rho^m_{1,k} + \rho^m_{1,l}$. In addition, we assume that anterograde mitochondria split in proportion to the cross sectional area of daughter branches: $\frac{\rho^+_{1,k}}{\rho^+_{1,l}} = \frac{r_k^2}{r_l^2} = \frac{\rho^m_{1,k}}{\rho^m_{1,l}}$. For Da Vinci trees (where $r_j^\alpha = r_k^\alpha + r_l^\alpha$ at each junction), this gives a simple relationship between the parent and daughter motile densities: $\rho^m_{1k} = \rho^m_{1j}(r_k^2/r_j^2)$. This implies that the linear density of motile mitochondria on each branch can be written in closed form:

$$\rho^m_{1,j} = \frac{2k_p r_j^2}{v r_0^2}, \tag{S.8}$$

where index 0 refers to the primary trunk.

For trees that do not obey Da Vinci scaling (*e.g.* $\alpha \neq 2$), the linear density of motile monomers must be computed recursively at each junction by starting with the primary trunk density and computing each successive pair of daughter branch densities as:

$$\rho^m_{1,k} = \rho^m_{1,j}\frac{r_k^2}{r_k^2 + r_l^2}; \;\; \rho^m_{1,l} = \rho^m_{1,j}\frac{r_l^2}{r_k^2 + r_l^2}. \tag{S.9}$$

Equations S.7 and S.9 together are used to compute the linear density of each cluster size on each individual branch of a tree.

The distribution of cluster sizes (plotted in Fig. 2a) is defined by averaging over the entire tree or subtree (ST) under consideration:

$$\rho_{i,\mathrm{ST}} = \left(\sum_{j\in \mathrm{ST}} \rho_{i,j} l_j\right) \Bigg/ \left(\sum_{j\in \mathrm{ST}} \sum_{i=1}^{\infty} \rho_{i,j} l_j\right). \tag{S.10}$$

## MOMENTS AND AVERAGES OF THE DISTRIBUTION

The overall linear density of mitochondrial clusters on branch $j$ is given by summing Eq. S.7 over all cluster sizes:

$$m_{0,j} = \sum_{i=1}^{\infty} \rho_{i,j} = \rho^s_{1,j} + \rho^m_{1,j} + \sum_{i=1}^{\infty}\rho_{i,j} - \rho_{1,j} = \frac{\rho^m_{1,j}}{2} + \frac{\rho^m_{1,j}(1+\alpha_j \rho^m_{1,j})}{2(1-\alpha_j\rho^m_{1,j})}. \tag{S.11}$$

Similarly, the linear density of individual mitochondrial units is given by the next moment of the distribution:

$$m_{1,j} = \sum_{i=1}^{\infty} i\rho_{i,j} = \rho^s_{1,j} + \rho^m_{1,j} + \sum_{i=1}^{\infty} i\rho_{i,j} - \rho_{1,j} = \frac{\rho^m_{1,j}}{2} + \frac{\rho^m_{1,j}(1+\alpha_j \rho^m_{1,j})}{2(1-\alpha_j\rho^m_{1,j})^2}, \tag{S.12}$$

We define the dilution factor $\xi_j = \rho^m_{1,j}/\rho^m_{1,0}$, which depends only on the tree structure (specifically, on the radii of all branches upstream of $j$). Additionally, we define the two dimensionless quantities $\hat{k}_p = \frac{k_p D_0}{v}$, and $u = \frac{A_u v}{r_0^\gamma D_0 k_b}$, where $D_0$ is the depth of the tree. This yields the following expressions:

$$\begin{aligned} \rho^m_{1,j} &= \xi_j \rho^m_{1,0} = \xi_j(2k_p/v) = 2\xi_j \hat{k}_p/D_0, \\ \alpha_j\rho^m_{1,j} &= vA_u/(2k_b r_j^\gamma) \times 2\xi_j\hat{k}_p/D_0 = \xi_j u \hat{k}_p r_0^\gamma/r_j^\gamma. \end{aligned} \tag{S.13}$$

Equations S.11, S.12, S.13 yield Eq. 3 in the main text. The above moments of the mitochondrial cluster distribution can be used to compute total mass, volume density, and average cluster size in different tree regions.

The total mitochondrial mass in tree T is given by

$$M_T = \sum_{j\in T} m_{1,j}\ell_j, \tag{S.14}$$

where $\ell_j$ is the length of the $j$-th branch. The average cluster size is defined as the ratio of the total mitochondrial mass divided by the total number of clusters in the tree:

$$\langle i\rangle_T = M_T / \sum_{j\in T} m_{0,j}\ell_j. \tag{S.15}$$

The mitochondrial volume density in a a given branch is given by $c_j = m_{1,j}/r_j^2$. The average mitochondrial volume density over a tree or subtree (T) is defined as the total mass divided by the tree volume:

$$c_T = M_T/V_T = \frac{M_T}{\sum_{j\in T} \ell_j r_j^2}. \tag{S.16}$$

## CANONICAL SOLUTION FOR $\gamma = 2$ ON BALANCED TREES

We next consider these metrics of the mitochondrial distribution for several special cases. A tree obeys Da Vinci's law if the cross sectional area is conserved across all junctions ($r_j^2 = r_k^2 + r_l^2$, for parent branch $j$ and daughter branches $k, l$). For such trees, Eq. S.8 implies that $\xi_j = r_j^2/r_0^2$. If we further assume that the fusion sensitivity exponent is set to $\gamma = 2$, the moments of the mitochondrial distribution (Eq. 3 in the main text) can be simplified to

$$\begin{aligned} m_{0,j} &= \frac{2r_j^2\hat{k}_p}{r_0^2 D_0} g[u\hat{k}_p], \\ m_{1,j} &= \frac{2r_j^2\hat{k}_p}{r_0^2 D_0} f[u\hat{k}_p]. \end{aligned} \tag{S.17}$$

As a result, the average cluster size (Eq. S.15) is given by

$$\langle i \rangle_{\text{T, DaVinci}} = \frac{f[u\hat{k}_p]}{g[u\hat{k}_p]} = \frac{(u\hat{k}_p)^2 - u\hat{k}_p + 2}{2(1 - u\hat{k}_p)}. \tag{S.18}$$

Thus, for Da Vinci trees, the average cluster size is independent of the tree topology or the specific choice of branch radii.

A balanced tree structure is one that both obeys Da Vinci's Law and splits sister branches such that cross-sectional area is proportional to the bushiness of the two subtrees which they support ($r_k^2/r_l^2 = B_k/B_l$ at each junction, where $B_k = L_k/D_k$ is the length divided by the depth of the subtree stemming from branch $k$). We note that a linear structure with a single branch is a trivial example of a balanced tree.

The depth of a subtree starting with parent branch $j$ is defined recursively [1] via the following relation:

$$D_j = \ell_j + \frac{L_k + L_l}{L_k/D_k + L_l/D_l}, \tag{S.19}$$

where $L_k$ is the total branch length in the daughter subtree stemming from branch $k$, and $D_k$ is the depth of that subtree. We note that for a subtree consisting of a single branch, or one where all branch tips are the same path-length from the root, the depth is equal to that path length. For more complicated tree structures, this recursive definition involves an average of inverse depth for the daughter subtrees, weighted by the total branch length in that tree.

Balanced trees allow for substantial simplification in the morphological features of the tree. Specifically, one can show for each junction that

$$\frac{r_k^2}{r_j^2} = \frac{L_k/D_k}{L_k/D_k + L_l/D_l}. \tag{S.20}$$

Suppose that the total tree volume for the subtree stemming from branch $k$ is given by $V_k = r_k^2 D_k$. This is trivially true for a subtree composed of a single branch, where $D_k = \ell_k$. We can then show by induction that the same simple expression for tree volume holds for all the upstream branches. For the full balanced tree with primary trunk 0, we have

$$V_0 = r_0^2 D_0. \tag{S.21}$$

This relation allows a simple universal expression for the total mitochondrial mass in a balanced tree (when $\gamma = 2$). Combining Eq. S.14, S.17, S.21 gives

$$M_{\text{T,balanced}} = 2\hat{k}_p f[u\hat{k}_p] \frac{\sum_j r_j^2 \ell_j}{V_0} = 2\hat{k}_p f[u\hat{k}_p] = 2\hat{k}_p \left[1 + \frac{1 + u\hat{k}_p}{(1 - u\hat{k}_p)^2}\right] \tag{S.22}$$

## SIMULATIONS OF MITOCHONDRIAL DYNAMICS IN DENDRITIC TREES

Stochastic simulations of mitochondrial transport, fusion, and fission were implemented on a network of one-dimensional edges. The network topology was taken from the dendritic arbor of a *Drosophila* HS neuron [1] (Fig. 1a), and a distal subtree was extracted for the simulations (Fig. 1c). The width of branches in the subtree were assigned by imposing the rules for balanced trees and non-dimensionalizing by setting $r_0 = 1$ in the primary trunk.

The simulations were implemented in Fortran 90. For each run, 500 single mitochondrial units are placed on the subtree, with the number initialized on each branch proportional to the branch volume ($v_j = l_j r_j^2$). Each mitochondrion was initialized in a motile state, walking either in the anterograde (away from root) or retrograde (towards root) direction. At every time step $\Delta t = 0.01$s, motile mitochondria moved a distance of $\pm v\Delta t$ along the branch, with the speed set to $v = 0.45\mu m/s$. Whenever an anterograde mitochondrion hit a terminal tip, it reversed and becomes retrograde until it reaches the root, where it disappeared. Anterograde mitochondria split at junctions in proportion to daughter branch area $r_j^2$. Aside from fusion, there was no interaction or exclusion between passing mitochondria.

New mitochondria were produced at the primary trunk with a constant rate $k_p = 0.1s^{-1}$. When a motile mitochondrion passed the tip of any mitochondrial cluster (or another motile mitochondrion) fusion was allowed to occur with probability: $P_{u,j} = A_u/r_j^\gamma$ and $\gamma = 2, 5$. All clusters containing more than one unit were assumed to remain stationary.

Any cluster with size $i > 1$ could undergo fission and release a single motile unit, with fission rate $k_b = 0.018s^{-1}$ from either end. Fission always produced one stationary unit or cluster plus one motile unit. A stationary mitochondrion could become motile again with the same rate $k_b$ in each direction. To achieve the steady state configuration, the simulations were run for $10^8$ steps.

## DENDRITIC ARBOR STRUCTURES

Figure S1a shows the skeletons of 10 dendritic arbors from *Drosophila* HS neurons. The arbor structures were extracted from confocal microscopy images following stochastic MultiColor FlipOut (MCFO) labeling of individual HS dendrites, as described in prior work [1]. The tree topologies used here are the same ones as were reported in Ref. [1]. For each tree, branch radii were imposed according to different scaling rules, as described in the main text. The results in Figure 3 used one example arbor structure (boxed in Figure S1a). Results in Figure 4 are averaged over all 10 structures.

Figures S1b-g show how the total mitochondrial mass and average cluster size vary between different tree structures that obey identical rules for the branch radii. We note that for balanced trees with fusion sensitivity $\gamma = 2$, the results are independent of the tree topology. For other branch width rules or radial-dependencies of fusion, different tree structures alter the statistics of the cluster distribution.

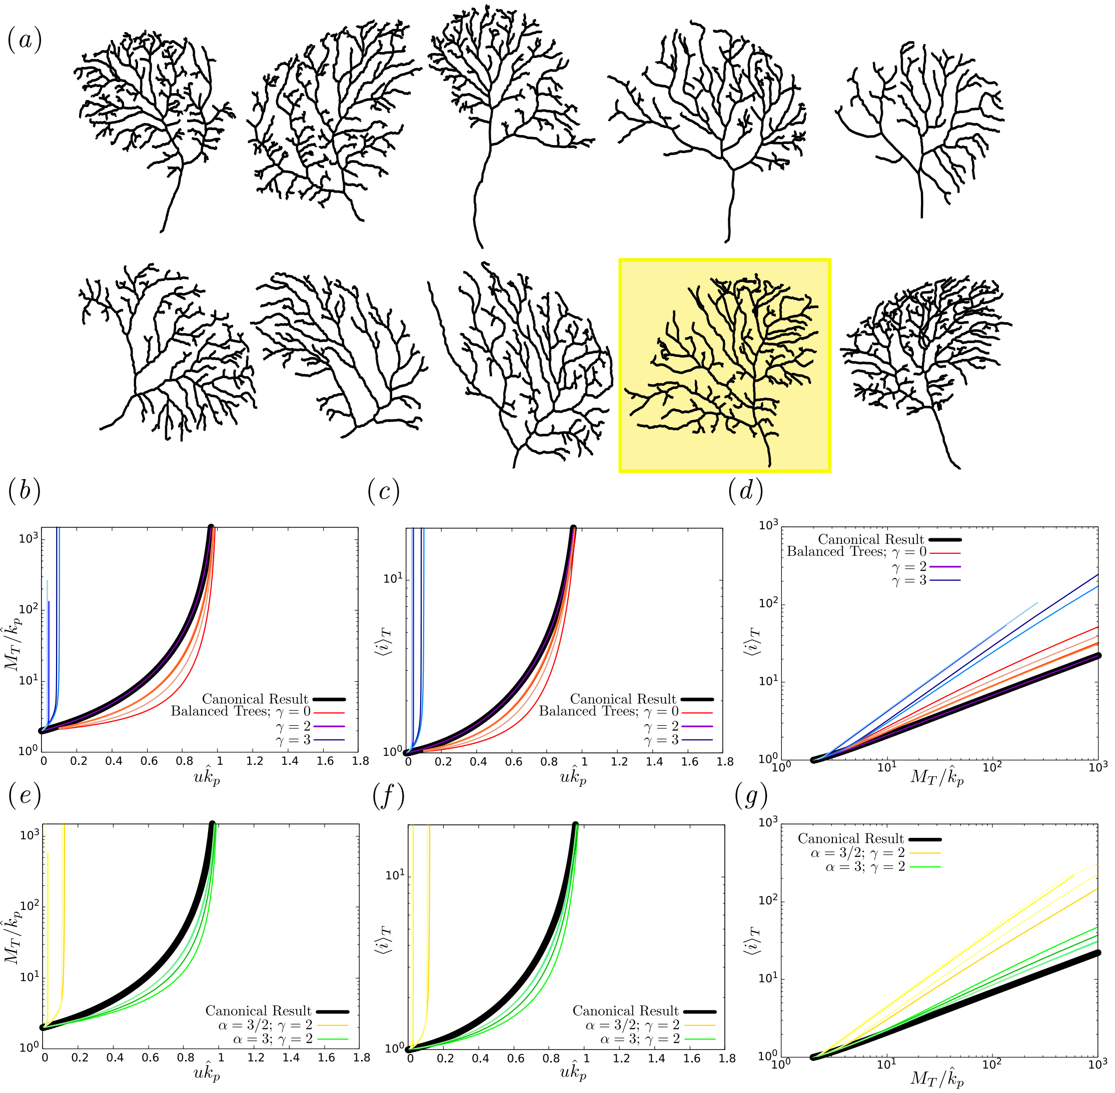


FIG. S1. $(a)$ Tree skeletons for the HS dendritic arbors from 10 individual neurons, with bushiness $B_0 \in [10.9, 21.8]$, average bushiness $\langle B_0 \rangle \sim 16$, RMS asymmetry in subtree length $\zeta_{L_0} \in [0.45, 0.56]$, and $\langle \zeta_{L_0} \rangle \sim 0.5$. Yellow box shows tree structure used in main text. $(b)$ Scaled total mitochondrial mass versus dimensionless parameter $u\hat{k}_p$, for 4 different balanced trees with fusion exponent $\gamma = 0$ (red curves), $\gamma = 2$ (purple lines) and $\gamma = 3$ (blue lines). $(c)$ and $(d)$ the same as in $(b)$ but for the average cluster size versus $u\hat{k}_p$ and the average cluster size versus the scaled mitochondrial mass. $(e)$ Scaled total mitochondrial mass versus $u\hat{k}_p$, for $\gamma = 2$ and different radial scaling with $\alpha = 3/2$ (yellow curves) and $\alpha = 3$ (green lines). $(f)$ and $(g)$ display the corresponding average cluster size versus $u\hat{k}_p$ and the average cluster size versus the scaled mitochondrial mass for unbalanced trees. In all cases the black lines corresponds to a linear geometry with $\gamma = 2$.

[1] E. J. Donovan, A. Agrawal, N. Liberman, J. I. Kalai, N. J. Chua, E. F. Koslover, and E. L. Barnhart, bioRxiv (in press at Cell Reports) (2022), 10.1101/2022.07.01.497972.
